# Supplementary material for: Exploration of Hexagonal, Layered Carbides and Nitrides as Ultra-High Temperature Ceramics
Source: arXiv:2508.18455 source file (2025-08-25)
Supplement: Supplementary file 1 [file SI.pdf]

# Supplemental Information: Exploration of Hexagonal, Layered Carbides and Nitrides as Ultra-High Temperature Ceramics

Kat Nykiel[1], Brian Wyatt[2], Babak Anasori[2], and Alejandro Strachan[1]

[1]School of Materials Engineering and Birck Nanotechnology Center, Purdue University
[2]School of Materials Engineering, Purdue University

February 10, 2025

## Zeta-Like Structure Generation

After applying rotations and translations to stacked MXene sheets, we obtain 16 unique zeta-like unit cell structures. All 16 of our zeta-like structures are shown in Figure 1. The structures are labeled with the Jagodzinski-Wyckoff notation discussed in the main text. Each row indicates the number of layers in the MXene sheet ($n$=1,2,3), and each column indicates the number of stacked MXenes in a given unit cell.

## Convergence Testing

In Figure 2, we show the c lattice parameter of the *hcch-hcch-hcch* $Ti_4N_3$ structure as a function of the kinetic energy cutoff and number of kpoints along the z axis. We see that at a kinetic energy cutoff of 550 eV and 10 kpoints along the z axis, the c lattice parameter is converged to within 0.01 Å. We use this kinetic energy cutoff in all geometric relaxations, and use a kpoint density of 1450 / $n_{atoms}$ to adjust for the different unit cell sizes.

## Melting Temperature Prediction

Desai and Strachan [1] construct their models from linear combinations of temperature-unit independent quantities, listed below in Eq. 1-4

$$\theta_0 = \frac{\hbar v_m}{k_b a} \tag{1}$$

$$\theta_1 = \frac{\hbar^2}{m a^2 k_b} \tag{2}$$

$$\theta_2 = \frac{a^3 G}{k_b} \tag{3}$$

$$\theta_3 = \frac{a^3 K}{k_b} \tag{4}$$

Here, $K$ and $G$ are the bulk and shear moduli, $a$ is the characteristic atomic distance, and $m$ is the mean atomic mass. To normalize to units of temperature, these expressions include the Boltzmann constant $k_b$ and Planck's constant $\hbar$. From these inputs with dimensions of temperature, we predict the melting temperature with PNNs B and C in Eq. 5 and 6, as well as the Lindemann melting criteria in Eq. 7.

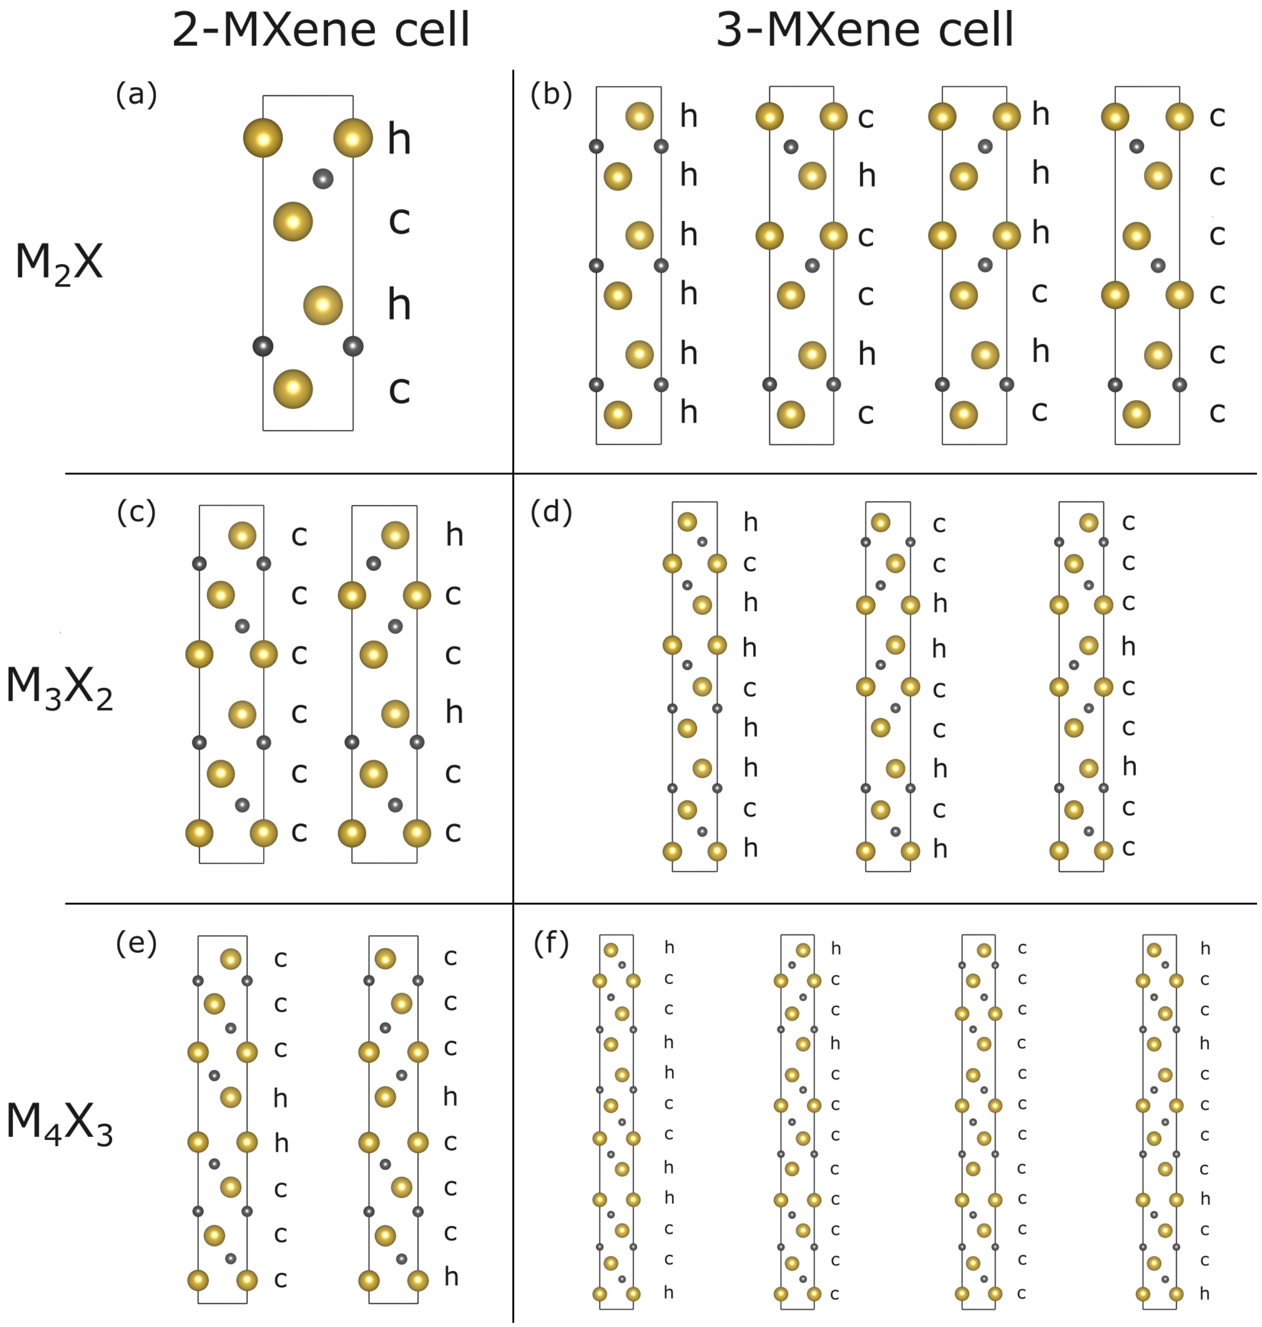


Figure 1: The 16 zeta-like structures investigated in this work.

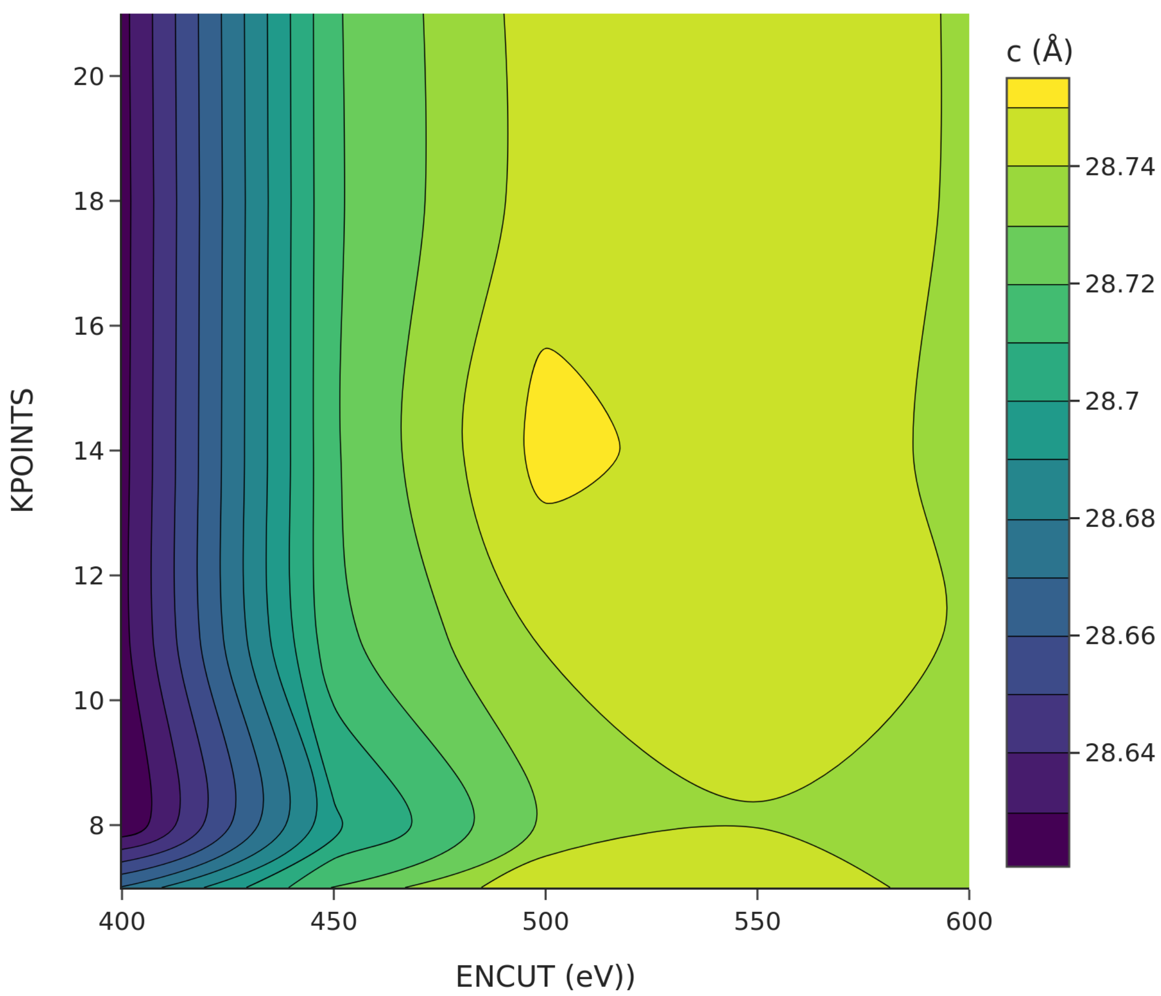


Figure 2: Convergence testing for the hcch-hcch-hcch $Ti_4N_3$ structure.

$$T_{\text{PNN B}} = 17.553\theta_0 + 0.001985\theta_2 \tag{5}$$

$$T_{\text{PNN C}} = 11.9034\theta_0 + 0.000499\theta_3 + 0.00796\frac{\theta_0^2}{\theta_1} \tag{6}$$

$$T_{\text{lind}} = C\frac{\theta_0^2}{\theta_1} = \frac{k_B}{9\hbar}f^2a^2mT_D^2 \tag{7}$$

In their work, Desai et al. found that PNN B and C had RMSE values of 530 K and 510 K applied to their test set. We expect that this method can provide a reasonable estimate of melting temperature for our zeta-like phases. When reporting melting temperature, in the results section, we take the average prediction of these three models.

## Validation

### Materials Project

To validate our computational methods, we compared our results to Materials Project, a large, carefully curated database of materials properties [2]. Using the Materials Project API, we identified 18 structures in Materials Project that are also contained within the set of 350 zeta-like structures in this work. Most of these structures are single-layer MXenes. These structures are reported below, with an asterisk (*) to indicate phases which also contain elastic data.

- Ta2C*: 164, mp-7088
- Ta2N*: 164, mp-10196
- Ti2C: 166, mp-1217106
- Hf3N2: 166, mp-1224388
- Nb4C3: 166, mp-1220515
- Nb2C*: 164, mp-2318
- Nb2N: 164, mp-1220726
- Mo4C3: 166, mp-1221488
- Mo2C: 164, mp-1221498
- Mo3C2: 164, mp-1221473
- Mo2N: 166, mp-1221525
- V4C3: 166, mp-1216471
- V2C*: 164, mp-1008632
- V4N3: 166, mp-1216472
- W2C*: 164, mp-1008625
- Sc2C: 164, mp-29941
- Cr2C: 164, mp-1226378
- Mn2N: 164, mp-1221793

For the 6 phases with elastic constants, we report both our calculated values and the Materials Project values in Table 1. The differences in elastic constants are likely due to the slight differences in pseudopotentials used between each set of calculations.

Table 1: Comparison of predicted elastic constants to Materials Project values.

| | Materials Project | | | This work | | |
|---|---|---|---|---|---|---|
| MXene | G (GPa) | K (GPa) | $T_D$ (K) | G (GPa) | K (GPa) | $T_D$ (K) |
| Nb2C | 62 | 223 | 394 | 69 | 220 | 414 |
| Ta2N | 118 | 270 | 387 | 118 | 271 | 387 |
| Ta2C | 146 | 260 | 431 | 147 | 258 | 433 |
| W2C | 156 | 315 | 437 | 159 | 315 | 441 |
| V2C | 100 | 219 | 623 | 102 | 219 | 630 |
| Sc2C | 9 | 71 | 223 | 13 | 73 | 265 |

Table 2: Summary of hc ordering properties

| hc ordering | $T_m$ (K) | $E_{hull}$ (eV/atom) | $Y$ (GPa) | $G$ (GPa) | $K$ (GPa) |
|---|---|---|---|---|---|
| hc-hc | 1900 | 0.16 | 200 | 76 | 210 |
| hh-hh-hh | 2300 | 0.13 | 260 | 100 | 210 |
| ch-cc-hc | 2000 | 0.16 | 220 | 82 | 220 |
| hh-hc-hc | 2100 | 0.13 | 240 | 91 | 200 |
| cc-cc-cc | 2000 | 0.16 | 220 | 83 | 220 |
| ccc-ccc | 2000 | 0.18 | 220 | 83 | 220 |
| hcc-hcc | 2200 | 0.20 | 260 | 98 | 240 |
| hch-hch-hch | 2400 | 0.16 | 280 | 110 | 210 |
| cch-hcc-hch | 2200 | 0.15 | 250 | 94 | 220 |
| ccc-hcc-hcc | 2200 | 0.19 | 240 | 92 | 230 |
| ccch-hccc | 2100 | 0.22 | 240 | 91 | 240 |
| ccch-ccch | 2200 | 0.21 | 240 | 93 | 220 |
| hcch-hcch-hcch | 2600 | 0.17 | 320 | 120 | 230 |
| hcch-cccc-cccc | 2100 | 0.20 | 230 | 88 | 220 |
| cccc-cccc-cccc | 2100 | 0.26 | 240 | 92 | 250 |
| hcch-cccc-hcch | 2300 | 0.19 | 280 | 110 | 230 |

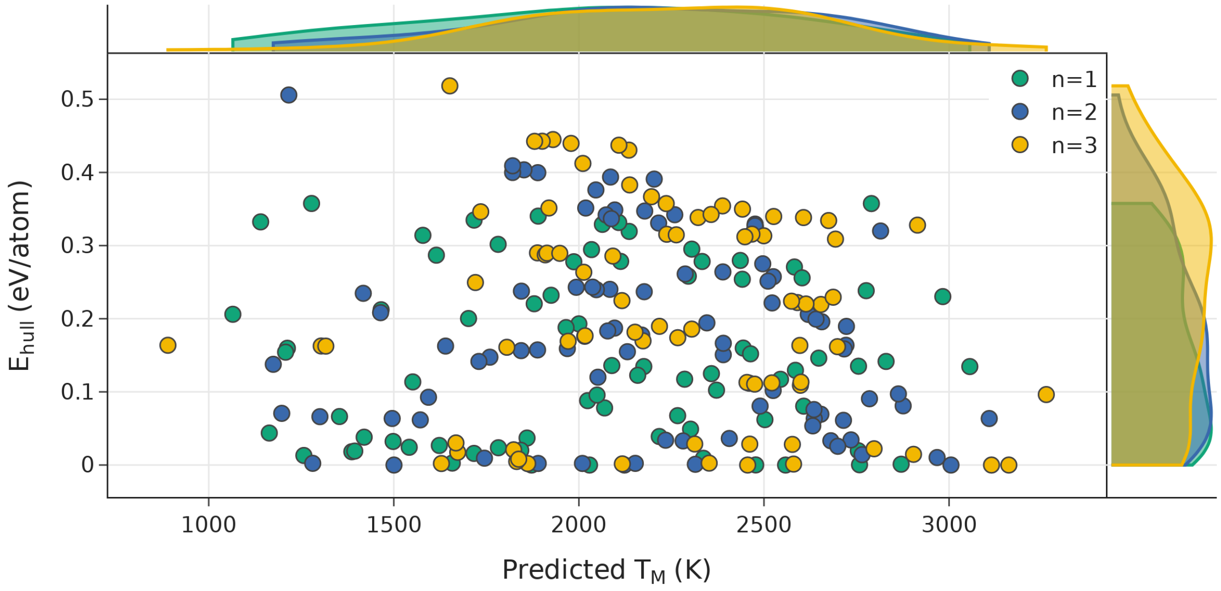


Figure 3: Distribution of UHTC properties, colored by the number of layers in the MXene structure.
